# Supplementary material for: Joint Energy-Bandwidth Allocation for Multi-User Channels with Cooperating Hybrid Energy Nodes
Source: arXiv:1611.05225 source file (2017-06-16)
Supplement: Supplementary file 1 [file appendixB.tex]

\appendices
\section{Proof of Theorem 2}
The authors of \cite{2012arXiv1208.3922H} give seven conditions for the function to satisfy, which guarantee optimality of ADMM. The objective function is sum of separable functions, and the constraints are linear which satisfy the problem structure in \cite{2012arXiv1208.3922H}. We will now verify these conditions for our problem in \eqref{epdef}-\eqref{epconst}.

\begin{enumerate}
\item The first condition is that the global minimum is attained and so is its dual optimal value. This holds since the problem is a convex problem.
\item The function in each variable can be written as sum of two parts. We refer to these two functions as the first part function   and the second part function. We split the functions as the first part functions being zero except that for $p_n^k$, where it is taken to be $-W_na_n^k \log(1+\frac{p_n^kH_n^k}{a_n^k})$. Thus, the rest of the functions are in the second part functions.

\item The first part functions are either constant, or are strictly convex and continuously differentiable on their domain with a uniform Lipschitz continuous gradient. We note that this holds trivially due to the functions splits mentioned in the last condition.
\item The epigraph of the second part functions is a polyhedral set. We note that the second part functions are a sum of a linear function and an indicator function, and thus their epigraph is a polyhedral set.
\item For given finite ${\cal Y}$ and finite $\psi({\cal P},{\cal L},{\cal R},{\cal S},{\cal G}, {\cal D}, {\cal U}, {\cal Y})$, the sum of the second part functions is finite in their domain. We note that  finite $\psi({\cal P},{\cal L},{\cal R},{\cal S},{\cal G}, {\cal D}, {\cal U}, {\cal Y})$ would mean that all indicator functions are zero and since all variables are bounded, the sum of the second part functions is bounded.
\item The matrix for constraint written as $\sum E_i x_i = q$ has full column rank $E_i$'s. We note that the corresponding $E_i$'s are single column with at-least one non-zero element and thus are all full column ranks.
\item The feasible sets for the variables are  compact polyhedral sets. This holds since feasible set of each variable is the real line.
\end{enumerate}
%We just showed that assumption A in [] holds for our problem formulation. Therefore we proved that ADMM converges to the optimal solution.
